# Supplementary material for: Size and shape of terrestrial animals
Source: arXiv:2602.00832 ancillary file (2026-01-31)
Supplement: Supplementary file 1 [file extended_data_tables.pdf]

# Extended tables

## Size and shape of terrestrial animals

Neelima Sharma<sup>\*1,2</sup> and Madhusudhan Venkadesan<sup>†2</sup>

<sup>1</sup>*Department of Cell & Developmental Biology, University College London, London, UK, WC1E 6BT*

<sup>2</sup>*Department of Mechanical Engineering & Materials Science, Yale University, New Haven, CT, USA*

---

<sup>\*</sup>`neelima.sharma@ucl.ac.uk`

<sup>†</sup>`m.venkadesan@yale.edu`

**Table E1. Information on data collected for 364 animals.** Table with animal names, frontal aspect ratio, mass, and the source from where animal photograph and mass were obtained.

| Animal                            | Aspect Ratio | Mass (kg) | Specimen photograph source | Specimen mass source |
|-----------------------------------|--------------|-----------|----------------------------|----------------------|
| <i>Chrysina macropus (m)</i>      | 4.24         | 0.00286   | M Dickman's collection     | Measured             |
| <i>Chrysina macropus (f)</i>      | 5.00         | 0.00180   | M Dickman's collection     | Measured             |
| <i>Chrysina spectabilis</i>       | 4.60         | 0.00270   | M Dickman's collection     | Measured             |
| <i>Chrysina guaymi</i>            | 3.61         | 0.00124   | M Dickman's collection     | Measured             |
| <i>Chrysina donthomasi</i>        | 3.87         | 0.00302   | M Dickman's collection     | Measured             |
| <i>Chrysina aurigans (6n)</i>     | 4.08         | 0.00241   | M Dickman's collection     | Measured             |
| <i>Chrysina aurigans (7n)</i>     | 4.43         | 0.00136   | M Dickman's collection     | Measured             |
| <i>Chrysina optima</i>            | 4.31         | 0.00086   | M Dickman's collection     | Measured             |
| <i>Chrysina batesi</i>            | 3.26         | 0.00202   | M Dickman's collection     | Measured             |
| <i>Chrysina resplendens</i>       | 3.06         | 0.00066   | M Dickman's collection     | Measured             |
| <i>Cerambycidae (11n)</i>         | 6.42         | 0.01238   | M Dickman's collection     | Measured             |
| <i>Goliathus orientalis (12n)</i> | 2.93         | 0.01552   | M Dickman's collection     | Measured             |
| <i>Goliathus orientalis (13n)</i> | 3.80         | 0.03232   | M Dickman's collection     | Measured             |
| <i>Macrodonia cervicornis</i>     | 7.66         | 0.01657   | M Dickman's collection     | Measured             |
| <i>Megasoma actaeon</i>           | 3.72         | 0.01808   | M Dickman's collection     | Measured             |
| <i>Cerambycidae (16n)</i>         | 12.23        | 0.02353   | M Dickman's collection     | Measured             |
| <i>Cerambycidae (17n)</i>         | 10.85        | 0.02182   | M Dickman's collection     | Measured             |
| <i>Cerambycidae (18n)</i>         | 6.60         | 0.00995   | M Dickman's collection     | Measured             |
| <i>Dynastes neptunus</i>          | 2.32         | 0.03363   | M Dickman's collection     | Measured             |
| <i>Chrysochroa buqueti</i>        | 5.05         | 0.00389   | M Dickman's collection     | Measured             |
| <i>Chrysochroa sp.</i>            | 4.80         | 0.00109   | M Dickman's collection     | Measured             |
| <i>Callospistus castelnaudi</i>   | 5.27         | 0.00367   | M Dickman's collection     | Measured             |
| <i>Callospistus wayersii</i>      | 4.48         | 0.00175   | M Dickman's collection     | Measured             |
| <i>Sternocera sternicornis</i>    | 2.79         | 0.00252   | M Dickman's collection     | Measured             |
| <i>Buprestidae (25n)</i>          | 5.35         | 0.00329   | M Dickman's collection     | Measured             |
| <i>Prosopocoilus cinnamomeus</i>  | 5.70         | 0.00524   | M Dickman's collection     | Measured             |
| <i>Prosopocoilus kannegieter</i>  | 4.11         | 0.00156   | M Dickman's collection     | Measured             |
| <i>Scarabaeidae (28n)</i>         | 9.39         | 0.00208   | M Dickman's collection     | Measured             |
| <i>Scarabaeidae (29n)</i>         | 5.86         | 0.00950   | M Dickman's collection     | Measured             |

**Table E1. Information on data collected for 364 animals.** Table with animal names, frontal aspect ratio, mass, and the source from where animal photograph and mass were obtained.

|                                       |      |            |                        |          |
|---------------------------------------|------|------------|------------------------|----------|
| <i>Buprestidae (30n)</i>              | 3.63 | 0.00650    | M Dickman's collection | Measured |
| <i>Cerambycidae (31n)</i>             | 6.08 | 0.00519    | M Dickman's collection | Measured |
| <i>Cerambycidae (32n)</i>             | 4.28 | 0.00349    | M Dickman's collection | Measured |
| <i>Scarabaeidae (33n)</i>             | 2.67 | 0.00206    | M Dickman's collection | Measured |
| <i>Scarabaeidae (34n)</i>             | 4.74 | 0.00439    | M Dickman's collection | Measured |
| <i>Elateridae (35n)</i>               | 5.37 | 0.00291    | M Dickman's collection | Measured |
| <i>Cerambycidae (36n)</i>             | 4.18 | 0.00316    | M Dickman's collection | Measured |
| <i>Scarabaeidae (37n)</i>             | 8.66 | 0.01319    | M Dickman's collection | Measured |
| <i>Scarabaeidae (38n)</i>             | 5.61 | 0.06827    | M Dickman's collection | Measured |
| <i>Titanus giganteum</i>              | 9.03 | 0.03553    | M Dickman's collection | Measured |
| <i>Antilocapra americana</i>          | 0.48 | 55.00000   | [1]                    | [1]      |
| <i>Babyrousa celebensis</i>           | 0.38 | 100.00000  | [1]                    | [1]      |
| <i>Bettongia lesueur</i>              | 0.38 | 0.84000    | [2]                    | [2]      |
| <i>Bos bison</i>                      | 0.35 | 679.00000  | [1]                    | [1]      |
| <i>Camelus bactrianus</i>             | 0.67 | 475.00000  | [1]                    | [1]      |
| <i>Capra nubiana</i>                  | 0.37 | 52.50000   | [1]                    | [1]      |
| <i>Capra pyrenaica</i>                | 0.34 | 27.25000   | [1]                    | [1]      |
| <i>Cephalophus hooki</i>              | 0.33 | 14.50000   | [1]                    | [1]      |
| <i>Cephalophus rufilatus</i>          | 0.80 | 10.50000   | [1]                    | [1]      |
| <i>Ceratotherium simum</i>            | 1.81 | 2425.00000 | [1]                    | [1]      |
| <i>Choeropsis liberiensis</i>         | 0.89 | 215.00000  | [1]                    | [1]      |
| <i>Dorcopsis muelleri</i>             | 0.98 | 5.90000    | [2]                    | [2]      |
| <i>Elephas maximus (1)</i>            | 0.45 | 4360.00000 | [1]                    | [1]      |
| <i>Equus africanus</i>                | 0.37 | 275.00000  | [1]                    | [1]      |
| <i>Gazella cora</i>                   | 0.69 | 17.50000   | [1]                    | [1]      |
| <i>Hylochoerus meinertzhageni (1)</i> | 1.09 | 187.50000  | [1]                    | [1]      |
| <i>Hylochoerus meinertzhageni (2)</i> | 0.61 | 187.50000  | [1]                    | [1]      |
| <i>Lasiornhinus latifrons</i>         | 1.00 | 0.02675    | [2]                    | [2]      |
| <i>Loxodonta cyclotis</i>             | 0.40 | 4350.00000 | [1]                    | [1]      |
| <i>Macropus giganteus</i>             | 0.74 | 53.50000   | [2]                    | [2]      |

**Table E1. Information on data collected for 364 animals.** Table with animal names, frontal aspect ratio, mass, and the source from where animal photograph and mass were obtained.

|                                  |      |           |                                   |                           |
|----------------------------------|------|-----------|-----------------------------------|---------------------------|
| <i>Madoqua guentheri</i>         | 0.53 | 4.05000   | [1]                               | [1]                       |
| <i>Neotragus livingstonianus</i> | 0.38 | 8.00000   | [1]                               | [1]                       |
| <i>Odocoileus hemionus</i>       | 0.36 | 72.50000  | [1]                               | [1]                       |
| <i>Osphranter antilopinus</i>    | 0.82 | 32.50000  | [2]                               | [2]                       |
| <i>Osphranter rufus</i>          | 0.59 | 54.50000  | [2]                               | [2]                       |
| <i>Ozotoceros bezoarticus</i>    | 0.27 | 28.00000  | [1]                               | [1]                       |
| <i>Porcula salvania</i>          | 0.57 | 8.15000   | [1]                               | [1]                       |
| <i>Pseudochirulus forbesi</i>    | 1.12 | 0.64250   | [2]                               | [2]                       |
| <i>Rucervus eldii</i>            | 0.37 | 92.50000  | [1]                               | [1]                       |
| <i>Rusa unicolor</i>             | 0.20 | 200.00000 | [1]                               | [1]                       |
| <i>Setonix brachyurus</i>        | 0.78 | 2.90000   | [2]                               | [2]                       |
| <i>Sminthopsis hirtipes</i>      | 1.98 | 0.01625   | [3]                               | [3]                       |
| <i>Sus scrofa</i>                | 0.54 | 182.00000 | [1]                               | [1]                       |
| <i>Syncerus caffer (1)</i>       | 0.72 | 625.00000 | [1]                               | [1]                       |
| <i>Syncerus nanus</i>            | 0.28 | 292.50000 | [1]                               | [1]                       |
| <i>Tapirus pinchaque</i>         | 0.51 | 175.00000 | [1]                               | [1]                       |
| <i>Tayassu pecari</i>            | 0.57 | 32.50000  | [1]                               | [1]                       |
| <i>Tragelaphus scriptus</i>      | 0.61 | 52.00000  | [1]                               | [1]                       |
| <i>Tragulus kanchil</i>          | 0.55 | 2.00000   | [1]                               | [1]                       |
| <i>Trichosurus vulpecula</i>     | 1.35 | 2.85000   | [2]                               | [2]                       |
| <i>Vicugna vicugna</i>           | 0.31 | 41.50000  | [1]                               | [1]                       |
| <i>Tragelaphus buxtoni</i>       | 0.29 | 235.00000 | [1]                               | [1]                       |
| <i>Grallaria blakei</i>          | 0.82 | 0.04250   | ML205512571, The Macaulay Library | [4]                       |
| <i>Turdus abyssinicus</i>        | 0.84 | 0.06140   | ML204353531, The Macaulay Library | [4]                       |
| <i>Bubo scandiacus (1)</i>       | 1.28 | 2.04100   | BIR025-00111, The Photo Ark       | [5], <a href="#">Link</a> |
| <i>Uraeginthus angolensis</i>    | 0.86 | 0.01300   | bir033-00589, The Photo Ark       | [5], <a href="#">Link</a> |
| <i>Panthera pardus saxicolor</i> | 0.68 | 41.00000  | ani105-00025, The Photo Ark       | [6], <a href="#">Link</a> |
| <i>Desmodus rotundus</i>         | 2.66 | 0.04400   | ani014-00048, The Photo Ark       | [5], <a href="#">Link</a> |
| <i>Burramys parvus</i>           | 1.70 | 0.01600   | ani051-00039, The Photo Ark       | [5], <a href="#">Link</a> |
| <i>Balaeniceps rex (1)</i>       | 0.70 | 5.98400   | bir030-00064, The Photo Ark       | [5], <a href="#">Link</a> |

**Table E1. Information on data collected for 364 animals.** Table with animal names, frontal aspect ratio, mass, and the source from where animal photograph and mass were obtained.

|                                     |      |            |                             |                           |
|-------------------------------------|------|------------|-----------------------------|---------------------------|
| <i>Phascolarctos cinereus</i>       | 0.79 | 1.15500    | ani088-00042, The Photo Ark | [5], <a href="#">Link</a> |
| <i>Fukomys damarensis</i>           | 1.66 | 0.14400    | ani012-00208, The Photo Ark | [6], <a href="#">Link</a> |
| <i>Elephas maximus</i> (2)          | 0.65 | 3305.12000 | ani018-00053, The Photo Ark | [5], <a href="#">Link</a> |
| <i>Varecia variegata</i>            | 1.00 | 3.85000    | ani040-00476, The Photo Ark | [5], <a href="#">Link</a> |
| <i>Leopardus pardalis</i>           | 0.69 | 17.00000   | ani019-00304, The Photo Ark | [5], <a href="#">Link</a> |
| <i>Dendromus melanotis</i>          | 1.60 | 0.00910    | ani012-00275, The Photo Ark | [5], <a href="#">Link</a> |
| <i>Perodicticus potto</i>           | 1.82 | 1.10000    | ani064-00095, The Photo Ark | [5], <a href="#">Link</a> |
| <i>Ursus arctos isabellinus</i>     | 0.71 | 340.00000  | bea020-00043, The Photo Ark | [6], <a href="#">Link</a> |
| <i>Gallicolumba luzonica</i>        | 0.94 | 0.18400    | bir052-00001, The Photo Ark | [5], <a href="#">Link</a> |
| <i>Aprosictus erythropterus</i>     | 1.35 | 0.13600    | bir037-00136, The Photo Ark | [5], <a href="#">Link</a> |
| <i>Tupaia palawanensis</i>          | 1.49 | 0.16805    | ani107-00029, The Photo Ark | [5], <a href="#">Link</a> |
| <i>Dendrocryna bicolor</i>          | 0.97 | 0.02879    | bir032-00325, The Photo Ark | [5], <a href="#">Link</a> |
| <i>Anas platyrhynchos</i> (1)       | 0.97 | 1.08200    | bir032-00362, The Photo Ark | [4]                       |
| <i>Anas platyrhynchos</i> (2)       | 0.87 | 1.08200    | bir032-00362, The Photo Ark | [4]                       |
| <i>Spheniscus mendiculus</i>        | 0.65 | 2.60000    | sce053-00080, The Photo Ark | [5], <a href="#">Link</a> |
| <i>Otus nigrorum</i>                | 0.96 | 0.24100    | bir025-00445, The Photo Ark | [4]                       |
| <i>Panthera onca</i> (1)            | 0.86 | 94.50000   | ani019-00519, The Photo Ark | [5], <a href="#">Link</a> |
| <i>Eudiptula minor</i>              | 1.12 | 1.15000    | bir036-00071, The Photo Ark | [5], <a href="#">Link</a> |
| <i>Hemigalus derbyanus</i>          | 0.73 | 0.12500    | ani062-00233, The Photo Ark | [5], <a href="#">Link</a> |
| <i>Chaetophractus vellerosus</i>    | 0.77 | 1.03000    | ani063-00059, The Photo Ark | [5], <a href="#">Link</a> |
| <i>Ammospermophilus harrisi</i>     | 1.33 | 0.12657    | ani072-00194, The Photo Ark | [5], <a href="#">Link</a> |
| <i>Otus lettia</i>                  | 0.76 | 0.12500    | bir070-00002, The Photo Ark | [4]                       |
| <i>Pheucticus melanocephalus</i>    | 1.42 | 0.03690    | bir067-00158, The Photo Ark | [5], <a href="#">Link</a> |
| <i>Ammodramus savannarum</i>        | 1.23 | 0.01725    | bir049-00104, The Photo Ark | [5], <a href="#">Link</a> |
| <i>Hylopetes alboniger</i>          | 1.66 | 0.25538    | ani072-00171, The Photo Ark | [5], <a href="#">Link</a> |
| <i>Chauna chavaria</i>              | 1.03 | 3.09000    | bir059-00359, The Photo Ark | [5], <a href="#">Link</a> |
| <i>Strix leptogrammica maingayi</i> | 1.07 | 0.95000    | bir025-00405, The Photo Ark | [4]                       |
| <i>Engystomops pustulosus</i>       | 2.02 | 0.00236    | ani078-00505, The Photo Ark | [5], <a href="#">Link</a> |
| <i>Botaurus lentiginosus</i>        | 0.86 | 0.60000    | bir053-00230, The Photo Ark | [5], <a href="#">Link</a> |
| <i>Sciurus niger</i>                | 0.86 | 0.80370    | ani072-00069, The Photo Ark | [5], <a href="#">Link</a> |

**Table E1. Information on data collected for 364 animals.** Table with animal names, frontal aspect ratio, mass, and the source from where animal photograph and mass were obtained.

|                                                 |      |         |                             |                           |
|-------------------------------------------------|------|---------|-----------------------------|---------------------------|
| <i>Pseudemys nelsoni</i>                        | 3.05 | 6.92919 | ENV020-00042, The Photo Ark | [5], <a href="#">Link</a> |
| <i>Anser cygnoides</i>                          | 0.77 | 3.45000 | BIR066-00007, The Photo Ark | [5], <a href="#">Link</a> |
| <i>Lophonetta specularioides specularioides</i> | 1.18 | 1.02150 | BIR060-00480, The Photo Ark | [4]                       |
| <i>Himantopus leucocephalus</i> (1)             | 0.46 | 0.19300 | BIR015-00172, The Photo Ark | [5], <a href="#">Link</a> |
| <i>Himantopus leucocephalus</i> (2)             | 0.62 | 0.19300 | BIR015-00171, The Photo Ark | [5], <a href="#">Link</a> |
| <i>Gyps africanus</i>                           | 0.99 | 0.03735 | BIR020-00085, The Photo Ark | [5], <a href="#">Link</a> |
| <i>Musophaga rossae</i>                         | 1.27 | 0.47500 | BIR033-00585, The Photo Ark | [5], <a href="#">Link</a> |
| <i>Sternotherus carinatus</i>                   | 2.93 | 0.92843 | ENV020-00044, The Photo Ark | [5], <a href="#">Link</a> |
| <i>Saguinus mystax</i>                          | 1.26 | 0.61800 | ANI099-00126, The Photo Ark | [5], <a href="#">Link</a> |
| <i>Mustela nigripes</i>                         | 0.94 | 0.90710 | ANI029-00078, The Photo Ark | [5], <a href="#">Link</a> |
| <i>Myiophonus caeruleus</i> ssp.                | 1.72 | 0.17900 | BIR064-00111, The Photo Ark | [5], <a href="#">Link</a> |
| <i>Rhinoclemmys melanosterna</i>                | 3.01 | 3.34900 | ANI080-00480, The Photo Ark | [5], <a href="#">Link</a> |
| <i>Xipholena punicea</i>                        | 0.68 | 0.07600 | BIR052-00107, The Photo Ark | [5], <a href="#">Link</a> |
| <i>Tringa melanoleuca</i>                       | 0.70 | 0.17010 | BIR015-00118, The Photo Ark | [5], <a href="#">Link</a> |
| <i>Phoenicopiterus ruber</i>                    | 0.73 | 4.10000 | BIR035-00056, The Photo Ark | [5], <a href="#">Link</a> |
| <i>Irena puella</i>                             | 1.03 | 0.07030 | BIR053-00252, The Photo Ark | [5], <a href="#">Link</a> |
| <i>Coscoroba coscoroba</i>                      | 0.98 | 5.40000 | BIR028-00027, The Photo Ark | [5], <a href="#">Link</a> |
| <i>Ardea alba</i>                               | 0.85 | 0.91200 | BIR009-00035, The Photo Ark | [5], <a href="#">Link</a> |
| <i>Oryctolagus cuniculus</i>                    | 1.29 | 2.15000 | ANI031-00127, The Photo Ark | [5], <a href="#">Link</a> |
| <i>Perameles gunni</i>                          | 1.38 | 0.64000 | ANI051-00047, The Photo Ark | [6], <a href="#">Link</a> |
| <i>Nycticorax nycticorax hoactli</i>            | 0.99 | 0.81000 | BIR011-00014, The Photo Ark | [4]                       |
| <i>Procyon cancrivorus nigripes</i>             | 0.88 | 6.00000 | ANI057-00032, The Photo Ark | [5]                       |
| <i>Meriones vinogradovi</i>                     | 1.69 | 0.00300 | ANI084-00203, The Photo Ark | [5], <a href="#">Link</a> |
| <i>Pygoscelis papua papua</i> (1)               | 0.64 | 5.95000 | BIR036-00094, The Photo Ark | [4]                       |
| <i>Pygoscelis papua papua</i> (2)               | 0.56 | 5.95000 | BIR036-00094, The Photo Ark | [4]                       |
| <i>Pocephalus gulielmi fantiensis</i>           | 0.70 | 0.27500 | BIR037-00259, The Photo Ark | [4]                       |
| <i>Aythya valisineria</i>                       | 1.17 | 0.86300 | BIR032-00488, The Photo Ark | [5], <a href="#">Link</a> |
| <i>Kinosternon leucostomum leucostomum</i>      | 2.70 | 0.24345 | ANI080-00214, The Photo Ark | [7]                       |

**Table E1. Information on data collected for 364 animals.** Table with animal names, frontal aspect ratio, mass, and the source from where animal photograph and mass were obtained.

|                                                  |      |           |                             |                           |
|--------------------------------------------------|------|-----------|-----------------------------|---------------------------|
| <i>Reithrodontomys megalotis</i>                 | 1.54 | 0.01103   | ANI012-00241, The Photo Ark | [5], <a href="#">Link</a> |
| <i>Pulsatrix perspicillata</i>                   | 1.11 | 0.67950   | BIR025-00175, The Photo Ark | [5], <a href="#">Link</a> |
| <i>Ursus americanus luteolus</i>                 | 0.71 | 224.00000 | BEA018-00019, The Photo Ark | [6], <a href="#">Link</a> |
| <i>Spilornis holospilus</i>                      | 0.55 | 0.85800   | BIR040-00225, The Photo Ark | [5], <a href="#">Link</a> |
| <i>Lipaugus vociferans</i>                       | 0.94 | 0.08700   | BIR067-00266, The Photo Ark | [5], <a href="#">Link</a> |
| <i>Tachycineta bicolor</i>                       | 1.28 | 0.01900   | BIR067-00138, The Photo Ark | [5], <a href="#">Link</a> |
| <i>Aythya fuligula</i>                           | 1.22 | 0.02846   | BIR060-00521, The Photo Ark | [5], <a href="#">Link</a> |
| <i>Indotestudo elongata</i>                      | 3.47 | 1.90315   | ANI080-00465, The Photo Ark | [5], <a href="#">Link</a> |
| <i>Callosciurus erythraeus</i>                   | 2.02 | 0.28323   | ANI072-00086, The Photo Ark | [5], <a href="#">Link</a> |
| <i>Numida meleagris</i>                          | 0.92 | 1.58757   | BIR057-00196, The Photo Ark | [5], <a href="#">Link</a> |
| <i>Malaclemys terrapin tequesta</i>              | 3.31 | 0.72000   | ANI080-00391, The Photo Ark | [6], <a href="#">Link</a> |
| <i>Taxidea taxus</i>                             | 1.17 | 7.84215   | ANI056-00019, The Photo Ark | [5], <a href="#">Link</a> |
| <i>Varanus rudicollis</i>                        | 2.53 | 4.53241   | ANI073-00238, The Photo Ark | [5], <a href="#">Link</a> |
| <i>Polytelis anthopeplus</i>                     | 1.06 | 0.17000   | BIR037-00141, The Photo Ark | [5], <a href="#">Link</a> |
| <i>Callimico goeldii</i>                         | 1.05 | 0.12002   | ANI040-00414, The Photo Ark | [5], <a href="#">Link</a> |
| <i>Ursus thibetanus (1)</i>                      | 1.09 | 99.71419  | BEA018-00024, The Photo Ark | [5], <a href="#">Link</a> |
| <i>Galago senegalensis senegalensis</i>          | 0.94 | 0.06800   | ANI099-00087, The Photo Ark | [5], <a href="#">Link</a> |
| <i>Corvus corax principalis</i>                  | 1.04 | 0.78500   | BIR041-00015, The Photo Ark | [4]                       |
| <i>Eliomys melanurus</i>                         | 2.30 | 0.12300   | ANI084-00141, The Photo Ark | [5], <a href="#">Link</a> |
| <i>Psittacus erithacus erithacus (1)</i>         | 0.83 | 0.33300   | BIR037-00121, The Photo Ark | [4]                       |
| <i>Psittacus erithacus erithacus (2)</i>         | 0.85 | 0.33300   | BIR037-00121, The Photo Ark | [4]                       |
| <i>Anas wyvilliana</i>                           | 1.51 | 0.58500   | BIR066-00010, The Photo Ark | [5], <a href="#">Link</a> |
| <i>Polytelis alexandrae</i>                      | 0.90 | 0.11340   | BIR037-00138, The Photo Ark | [5], <a href="#">Link</a> |
| <i>Strigocuscus gymnotis</i>                     | 1.10 | 2.70500   | ANI051-00198, The Photo Ark | [5], <a href="#">Link</a> |
| <i>Ketupa ketupu ketupu</i>                      | 0.85 | 1.29300   | BIR025-00442, The Photo Ark | [4]                       |
| <i>Deroplatys lobata</i>                         | 2.15 | 0.02830   | INS004-00043, The Photo Ark | <a href="#">Link</a>      |
| <i>Peromyscus polionotus al-<br/>lophrys (1)</i> | 1.48 | 0.00593   | ESA002-00386, The Photo Ark | [5], <a href="#">Link</a> |
| <i>Ciccaba huhula huhula</i>                     | 1.41 | 0.37000   | BIR070-00095, The Photo Ark | [4]                       |

**Table E1. Information on data collected for 364 animals.** Table with animal names, frontal aspect ratio, mass, and the source from where animal photograph and mass were obtained.

|                                                  |      |           |                             |                           |
|--------------------------------------------------|------|-----------|-----------------------------|---------------------------|
| <i>Ciconia ciconia ciconia</i>                   | 0.39 | 3.44800   | BIR030-00049, The Photo Ark | [4]                       |
| <i>Graptemys flavimaculata</i>                   | 2.98 | 0.92843   | ESA002-00281, The Photo Ark | [5], <a href="#">Link</a> |
| <i>Grus americana</i>                            | 0.50 | 8.50000   | ESA001-00520, The Photo Ark | [5], <a href="#">Link</a> |
| <i>Dipsosaurus dorsalis</i>                      | 1.84 | 0.06601   | ANI073-00089, The Photo Ark | [5], <a href="#">Link</a> |
| <i>Eudytes chrysolophus</i>                      | 0.56 | 5.50000   | BIR036-00087, The Photo Ark | [5], <a href="#">Link</a> |
| <i>Microtus socialis nikolaevi</i>               | 1.01 | 0.00210   | ANI084-00253, The Photo Ark | [5], <a href="#">Link</a> |
| <i>Acomys spinosissimus</i>                      | 1.22 | 0.02650   | ANI012-00446, The Photo Ark | [5], <a href="#">Link</a> |
| <i>Podiceps nigricollis</i>                      | 1.73 | 0.02615   | BIR059-00178, The Photo Ark | [5], <a href="#">Link</a> |
| <i>Neochen jubata</i>                            | 0.92 | 1.25000   | BIR060-00338, The Photo Ark | [5], <a href="#">Link</a> |
| <i>Scaphidura oryzivora</i>                      | 1.26 | 0.18400   | BIR014-00065, The Photo Ark | [4]                       |
| <i>Gonocephalus grandis</i>                      | 2.22 | 0.09383   | ANI073-00634, The Photo Ark | [5], <a href="#">Link</a> |
| <i>Sciurus carolinensis carolinensis</i>         | 1.65 | 0.54400   | ANI072-00078, The Photo Ark | [6], <a href="#">Link</a> |
| <i>Bubo lacteus</i>                              | 0.89 | 1.70400   | BIR025-00238, The Photo Ark | [5], <a href="#">Link</a> |
| <i>Petaurus breviceps</i>                        | 3.22 | 0.04929   | ANI051-00085, The Photo Ark | [5], <a href="#">Link</a> |
| <i>Rollulus rouloul</i>                          | 1.41 | 0.23200   | BIR053-00070, The Photo Ark | [5], <a href="#">Link</a> |
| <i>Amazona rhodocorytha</i>                      | 0.93 | 0.50000   | BIR037-00173, The Photo Ark | [5], <a href="#">Link</a> |
| <i>Peromyscus polionotus al-<br/>lophrys</i> (2) | 2.05 | 0.00593   | ESA001-00432, The Photo Ark | [5], <a href="#">Link</a> |
| <i>Brachylagus idahoensis</i>                    | 1.05 | 0.43119   | ESA002-00199, The Photo Ark | [5], <a href="#">Link</a> |
| <i>Sus philippensis mindanensis</i>              | 0.42 | 190.79230 | ANI054-00042, The Photo Ark | [5], <a href="#">Link</a> |
| <i>Oriolus larvatus tibicen</i>                  | 1.12 | 0.07240   | BIR053-00127, The Photo Ark | [5], <a href="#">Link</a> |
| <i>Thallomys paeudulus</i>                       | 1.70 | 0.00265   | ANI084-00219, The Photo Ark | [5], <a href="#">Link</a> |
| <i>Agalychnis lemur</i> (1)                      | 2.14 | 0.00200   | ANI110-00281, The Photo Ark | <a href="#">Link</a>      |
| <i>Agalychnis lemur</i> (2)                      | 2.14 | 0.00200   | ANI110-00281, The Photo Ark | <a href="#">Link</a>      |
| <i>Cyrtonyx montezumae</i>                       | 0.98 | 0.19500   | BIR045-00089, The Photo Ark | [5], <a href="#">Link</a> |
| <i>Neotoma albigula</i>                          | 1.51 | 0.10330   | ANI012-00376, The Photo Ark | [5], <a href="#">Link</a> |
| <i>Bubulcus ibis</i>                             | 0.82 | 0.22000   | BIR009-00047, The Photo Ark | [5], <a href="#">Link</a> |
| <i>Macropus rufogriseus</i>                      | 0.99 | 3.19921   | ANI051-00057, The Photo Ark | [5], <a href="#">Link</a> |
| <i>Glyptemys muhlenbergii</i>                    | 1.89 | 0.11000   | ESA001-00387, The Photo Ark | [8]                       |



**Table E1. Information on data collected for 364 animals.** Table with animal names, frontal aspect ratio, mass, and the source from where animal photograph and mass were obtained.

|                                      |      |             |                                       |                           |
|--------------------------------------|------|-------------|---------------------------------------|---------------------------|
| <i>Megascops asio floridanus</i>     | 0.84 | 0.18050     | BIR025-00267, The Photo Ark           | [4]                       |
| <i>Tyto longimembris chinensis</i>   | 0.86 | 0.34150     | BIR070-00005, The Photo Ark           | [4]                       |
| <i>Asio clamator forbesi</i>         | 0.70 | 0.48500     | BIR025-00306, The Photo Ark           | [5], <a href="#">Link</a> |
| <i>Lepus granatensis granatensis</i> | 1.93 | 2.32394     | ANI031-00196, The Photo Ark           | [5], <a href="#">Link</a> |
| <i>Gymnobelideus leadbeateri</i>     | 2.08 | 0.03778     | ANI069-00019, The Photo Ark           | [5], <a href="#">Link</a> |
| <i>Aphelocoma coerulescens</i>       | 0.80 | 0.07700     | BIR031-00088, The Photo Ark           | [5], <a href="#">Link</a> |
| <i>Nyctanassa violacea (1)</i>       | 0.87 | 0.71600     | BIR011-00008, The Photo Ark           | [5], <a href="#">Link</a> |
| <i>Tolypeutes matacus</i>            | 0.59 | 1.30347     | ANI063-00028, The Photo Ark           | [5], <a href="#">Link</a> |
| <i>Parabuteo unicinctus harrisi</i>  | 0.70 | 0.73500     | BIR024-00083, The Photo Ark           | [5], <a href="#">Link</a> |
| <i>Pygoscelis papua ellsworthii</i>  | 0.87 | 8.50000     | BIR036-00063, The Photo Ark           | [5], <a href="#">Link</a> |
| <i>Bison bison</i>                   | 0.53 | 157.50000   | ANI082-00135, The Photo Ark           | [5], <a href="#">Link</a> |
| <i>Buteo jamaicensis umbrinus</i>    | 0.88 | 0.79500     | BIR024-00188, The Photo Ark           | [5], <a href="#">Link</a> |
| <i>Nycticebus javanicus</i>          | 2.46 | 0.67500     | ANI094-00024, The Photo Ark           | [5], <a href="#">Link</a> |
| <i>Lagothrix lagotricha</i>          | 1.13 | 6.50000     | ANI106-00089, The Photo Ark           | [6], <a href="#">Link</a> |
| <i>Salticidae</i>                    | 5.05 | 0.00003     | Bengaluru, India                      | Measured                  |
| <i>Periplaneta americana</i>         | 5.94 | 0.00005     | Bengaluru, India                      | Measured                  |
| <i>Raphus cucullatus</i>             | 0.69 | 13.75000    | Peabody museum display                | [9]                       |
| <i>Stegosaurus</i>                   | 0.71 | 1780.00000  | Peabody museum display                | [10]                      |
| <i>Deinonychus</i>                   | 0.55 | 85.00000    | Peabody museum display                | [11]                      |
| <i>Camarasaurus</i>                  | 0.82 | 22679.00000 | Peabody museum display                | [11]                      |
| <i>Camptosaurus</i>                  | 0.67 | 550.00000   | Peabody museum display                | [11]                      |
| <i>Homo sapiens</i>                  | 0.29 | 55.00000    | Self                                  | Measured                  |
| <i>Callichroma auricomum (4j)</i>    | 3.99 | 0.00142     | Peabody Entomology Catalog No. 971790 | Measured                  |
| <i>Trachyderes succinctus</i>        | 1.22 | 0.00056     | Peabody Entomology Catalog No. 972107 | Measured                  |
| <i>Rosenbergia straussi</i>          | 1.20 | 0.00707     | Peabody Entomology Catalog No. 972101 | Measured                  |
| <i>Euryphagus pictus</i>             | 3.95 | 0.00068     | Peabody Entomology Catalog No. 971892 | Measured                  |
| <i>Nicrophorus tomentosus</i>        | 3.32 | 0.00076     | Peabody Entomology Catalog No. 972013 | Measured                  |
| <i>Neandra brunnea</i>               | 3.58 | 0.00018     | Peabody Entomology Catalog No. 971901 | Measured                  |
| <i>Eleodes</i>                       | 2.58 | 0.00111     | Peabody Entomology Catalog No. 971787 | Measured                  |
| <i>Eupoecila australasiae</i>        | 2.52 | 0.00078     | Peabody Entomology Catalog No. 972110 | Measured                  |

**Table E1. Information on data collected for 364 animals.** Table with animal names, frontal aspect ratio, mass, and the source from where animal photograph and mass were obtained.

|                                       |      |           |                                       |            |
|---------------------------------------|------|-----------|---------------------------------------|------------|
| <i>Unknown (12j)</i>                  | 3.55 | 0.00030   | Peabody Entomology Catalog No. 971784 | Measured   |
| <i>Unknown (13j)</i>                  | 3.96 | 0.00159   | Peabody Entomology Catalog No. 971788 | Measured   |
| <i>Pelidnota punctata</i>             | 1.41 | 0.00162   | Peabody Entomology Catalog No. 972109 | Measured   |
| <i>Anoplophora glabripennis</i>       | 3.56 | 0.00132   | Peabody Entomology Catalog No. 972106 | Measured   |
| <i>Sternocera boucardi</i>            | 3.09 | 0.00492   | Peabody Entomology Catalog No. 971791 | Measured   |
| <i>Hycleus</i>                        | 3.90 | 0.00068   | Peabody Entomology Catalog No. 971894 | Measured   |
| <i>Calosoma senegalense</i>           | 5.15 | 0.00109   | Peabody Entomology Catalog No. 972536 | Measured   |
| <i>Carabidae</i>                      | 2.38 | 0.00099   | Peabody Entomology Catalog No. 972531 | Measured   |
| <i>Lucanidae odontolabis</i>          | 1.95 | 0.00329   | Peabody Entomology Catalog No. 972539 | Measured   |
| <i>Xylotrupes sp.</i>                 | 2.22 | 0.01112   | Peabody Entomology Catalog No. 971781 | Measured   |
| <i>Elateroidea</i>                    | 4.65 | 0.00554   | Peabody Entomology Catalog No. 971783 | Measured   |
| <i>Chalcosoma atlas</i>               | 2.72 | 0.01674   | Peabody Entomology Catalog No. 971789 | Measured   |
| <i>Acrocinus longimanus</i>           | 3.79 | 0.01030   | Peabody Entomology Catalog No. 972104 | Measured   |
| <i>Callichroma auricomum (26j)</i>    | 4.13 | 0.00142   | Peabody Entomology Catalog No. 971790 | Measured   |
| <i>Chrysochroa fulminans</i>          | 1.37 | 0.00118   | Peabody Entomology Catalog No. 971785 | Measured   |
| <i>Atilax paludinosus</i>             | 0.61 | 3.25000   | [12]                                  | [12]       |
| <i>Canis latrans</i>                  | 0.61 | 11.75000  | [12]                                  | [12]       |
| <i>Conepatus humboldtii</i>           | 0.79 | 1.50000   | [12]                                  | [12]       |
| <i>Crocuta crocuta</i>                | 0.44 | 50.00000  | [12]                                  | [12]       |
| <i>Hyaena hyaena</i>                  | 0.63 | 33.50000  | [12]                                  | [12]       |
| <i>Panthera leo</i>                   | 0.50 | 173.50000 | [12]                                  | [12]       |
| <i>Panthera onca (2)</i>              | 0.53 | 76.00000  | [12]                                  | [12]       |
| <i>Panthera uncia</i>                 | 0.71 | 37.00000  | [12]                                  | [12]       |
| <i>Ursus thibetanus (2)</i>           | 0.82 | 117.50000 | [12]                                  | [12]       |
| <i>Mixophyes fasciolatus</i>          | 3.72 | 0.02500   | ANI078-00350, The Photo Ark           | [13]       |
| <i>Scaphiophryne gottlebei (1)</i>    | 3.15 | 0.00615   | ANI078-00445, The Photo Ark           | [14]       |
| <i>Scaphiophryne gottlebei (2)</i>    | 3.46 | 0.00615   | ANI078-00445, The Photo Ark           | [14]       |
| <i>Hogna helluo or Tigrosa helluo</i> | 2.82 | 0.30000   | INS006-00088, The Photo Ark           | [15]       |
| <i>Vini australis</i>                 | 1.67 | 0.04950   | BIR068-00040, The Photo Ark           | [16], Link |
| <i>Dendrobates tinctorius</i>         | 4.55 | 0.00636   | ANI078-00518, The Photo Ark           | [17]       |

**Table E1. Information on data collected for 364 animals.** Table with animal names, frontal aspect ratio, mass, and the source from where animal photograph and mass were obtained.

|                                                        |      |            |                             |                           |
|--------------------------------------------------------|------|------------|-----------------------------|---------------------------|
| <i>Batagur affinis affinis</i>                         | 2.93 | 10.04000   | ANI104-00083, The Photo Ark | [18]                      |
| <i>Bufotes viridis</i> or <i>Pseudepidalea viridis</i> | 1.68 | 0.05500    | ANI078-00367, The Photo Ark | [19]                      |
| <i>Hierodula membranacea</i>                           | 3.08 | 0.00120    | INS004-00100, The Photo Ark | [20]                      |
| <i>Bufo melanostictus</i>                              | 3.84 | 0.02185    | ANI101-00196, The Photo Ark | [21]                      |
| <i>Aphonopelma hentzi</i>                              | 3.00 | 0.00480    | INS006-00133, The Photo Ark | [22]                      |
| <i>Ceratobatrachus guentheri</i>                       | 2.34 | 0.00350    | ANI071-00355, The Photo Ark | [23]                      |
| <i>Bombina orientalis</i>                              | 3.81 | 0.00864    | ANI101-00474, The Photo Ark | [24]                      |
| <i>Syncerus caffer</i> (2)                             | 0.45 | 567.50000  | Field Museum of Chicago     | [6], <a href="#">Link</a> |
| <i>Pelecanus conspicillatus</i>                        | 0.68 | 5.40000    | Field Museum of Chicago     | [6], <a href="#">Link</a> |
| <i>Babyrousa babyrussa</i>                             | 0.35 | 71.50000   | Field Museum of Chicago     | [6], <a href="#">Link</a> |
| <i>Oryx gazella beisa</i>                              | 0.20 | 210.00000  | Field Museum of Chicago     | [6], <a href="#">Link</a> |
| <i>Cephalophus nigrifrons</i>                          | 0.31 | 16.00000   | Field Museum of Chicago     | [25]                      |
| <i>Onychogalea fraenata</i>                            | 0.42 | 6.00000    | Field Museum of Chicago     | [6], <a href="#">Link</a> |
| <i>Pelecanus occidentalis</i>                          | 0.83 | 3.50000    | Field Museum of Chicago     | [6], <a href="#">Link</a> |
| <i>Equus burchelli</i> (1)                             | 0.21 | 280.00000  | Field Museum of Chicago     | [6], <a href="#">Link</a> |
| <i>Equus burchelli</i> (2)                             | 0.25 | 280.00000  | Field Museum of Chicago     | [6], <a href="#">Link</a> |
| <i>Anas cyanoptera</i>                                 | 0.85 | 0.38550    | Field Museum of Chicago     | [6], <a href="#">Link</a> |
| <i>Tayassu tajacu</i>                                  | 0.36 | 20.00000   | Field Museum of Chicago     | [6], <a href="#">Link</a> |
| <i>Mammuthus columbi</i>                               | 0.55 | 9500.00000 | Field Museum of Chicago     | [26]                      |
| <i>Vombatus ursinus</i>                                | 0.96 | 27.50000   | Field Museum of Chicago     | [6], <a href="#">Link</a> |
| <i>Ovis dalli dalli</i>                                | 0.26 | 79.50000   | Field Museum of Chicago     | [6], <a href="#">Link</a> |
| <i>Deinonychus antirrhopus</i>                         | 0.44 | 67.50000   | Field Museum of Chicago     | [27]                      |
| <i>Raphus cucullatus</i>                               | 0.67 | 10.20000   | Field Museum of Chicago     | [28]                      |
| <i>Aptenodytes forsteri</i> (1)                        | 0.36 | 29.50000   | Field Museum of Chicago     | [6], <a href="#">Link</a> |
| <i>Aptenodytes forsteri</i> (2)                        | 0.28 | 29.50000   | Field Museum of Chicago     | [6], <a href="#">Link</a> |
| <i>Galapagos Land Tortoise</i>                         | 2.61 | 250.00000  | Field Museum of Chicago     | Field Museum plate        |
| <i>Theropithecus gelada</i>                            | 0.47 | 17.00000   | Field Museum of Chicago     | [6], <a href="#">Link</a> |
| <i>Hylochoerus meinertzhageni</i> (3)                  | 0.54 | 227.50000  | Field Museum of Chicago     | [6], <a href="#">Link</a> |
| <i>Glyptodon clavipes</i>                              | 0.82 | 2000.00000 | Field Museum of Chicago     | [29]                      |

**Table E1. Information on data collected for 364 animals.** Table with animal names, frontal aspect ratio, mass, and the source from where animal photograph and mass were obtained.

|                                 |      |            |                               |                           |
|---------------------------------|------|------------|-------------------------------|---------------------------|
| <i>Gyps fulvus</i>              | 0.82 | 7.35000    | Field Museum of Chicago       | [4]                       |
| <i>Hemitragus jemlahicus</i>    | 0.29 | 63.00000   | Field Museum of Chicago       | [6], <a href="#">Link</a> |
| <i>Arctonyx collaris</i>        | 0.43 | 10.50000   | Field Museum of Chicago       | [6], <a href="#">Link</a> |
| <i>Hyracotherium sp.</i>        | 0.43 | 30.75000   | Field Museum of Chicago       | [30]                      |
| <i>Aptenodytes patagonicus</i>  | 0.52 | 13.30000   | Field Museum of Chicago       | [6], <a href="#">Link</a> |
| <i>Varanus komodoensis</i>      | 1.47 | 165.00000  | Field Museum of Chicago       | [6], <a href="#">Link</a> |
| <i>Chrysocyon brachyurus</i>    | 0.28 | 21.50000   | Field Museum of Chicago       | [6], <a href="#">Link</a> |
| <i>Mammut americanum</i>        | 0.62 | 6500.00000 | Field Museum of Chicago       | [26]                      |
| <i>Megaloceros giganteus</i>    | 0.20 | 600.00000  | Field Museum of Chicago       | [31]                      |
| <i>Megapodes</i>                | 0.71 | 1.61250    | Field Museum of Chicago       | [6], <a href="#">Link</a> |
| <i>Myrmecobius fasciatus</i>    | 1.04 | 0.52600    | Field Museum of Chicago       | [6], <a href="#">Link</a> |
| <i>Ophiacodon mirus</i>         | 3.24 | 128.00000  | Field Museum of Chicago       | [32]                      |
| <i>Protoceratops andrewsi</i>   | 1.79 | 75.50000   | Field Museum of Chicago       | [33]                      |
| <i>Quetzalcoatlus northropi</i> | 0.52 | 544.00000  | Field Museum of Chicago       | [34]                      |
| <i>Vulpes vulpes</i>            | 0.48 | 8.50000    | Field Museum of Chicago       | [6], <a href="#">Link</a> |
| <i>Oreamnos americanus</i>      | 0.34 | 69.30000   | Field Museum of Chicago       | [6], <a href="#">Link</a> |
| <i>Balaeniceps rex</i> (2)      | 0.42 | 5.98400    | Field Museum of Chicago       | [4]                       |
| <i>Diomedea albatrus</i>        | 0.83 | 4.41100    | Field Museum of Chicago       | [4]                       |
| <i>Bubo scandiacus</i> (2)      | 0.41 | 2.09850    | Field Museum of Chicago       | [4]                       |
| <i>Stegosaurus stenops</i>      | 0.56 | 1560.00000 | Field Museum of Chicago       | [35]                      |
| <i>Alcelaphus buselaphus</i>    | 0.21 | 137.50000  | Field Museum of Chicago       | [6], <a href="#">Link</a> |
| <i>Tyrannosaurus rex</i> (1)    | 0.89 | 6000.00000 | Field Museum of Chicago       | [36]                      |
| <i>Teleoceras major</i>         | 0.96 | 1500.00000 | Field Museum of Chicago       | [37]                      |
| <i>Terrapene carolina</i>       | 3.32 | 0.36250    | Field Museum of Chicago       | [38]                      |
| <i>Tiktaalik roseae</i>         | 2.50 | 6.94000    | Field Museum of Chicago       | [39]                      |
| <i>Triceratops horridus</i>     | 1.46 | 7045.50000 | Field Museum of Chicago       | [33]                      |
| <i>Phacochoerus aethiopicus</i> | 0.28 | 87.50000   | Field Museum of Chicago       | [6], <a href="#">Link</a> |
| <i>Hemiptera</i> (x4)           | 2.74 | 0.00005    | Collected in Bengaluru, India | Measured                  |
| <i>Orthoptera</i> (i1)          | 2.50 | 0.00007    | Collected in Bengaluru, India | Measured                  |
| <i>Orthoptera</i> (i2)          | 2.98 | 0.00044    | Collected in Bengaluru, India | Measured                  |

**Table E1. Information on data collected for 364 animals.** Table with animal names, frontal aspect ratio, mass, and the source from where animal photograph and mass were obtained.

|                                                    |      |           |                                                    |                                            |
|----------------------------------------------------|------|-----------|----------------------------------------------------|--------------------------------------------|
| <i>Rhea americana</i>                              | 0.47 | 23.00000  | <a href="#">ML711913</a> , The Macaulay Library    | <a href="#">[4]</a>                        |
| <i>Passerina leclancherii</i>                      | 1.17 | 0.01400   | <a href="#">ML714528</a> , The Macaulay Library    | <a href="#">[4]</a>                        |
| <i>Smutsornis africanus/ Rhinoptilus africanus</i> | 0.50 | 0.08750   | <a href="#">ML705140</a> , The Macaulay Library    | <a href="#">[4]</a>                        |
| <i>Ciconia abdimii</i>                             | 0.55 | 1.39800   | <a href="#">ML705833</a> , The Macaulay Library    | <a href="#">[4]</a>                        |
| <i>Leptoptilos crumenifer</i>                      | 0.37 | 6.32500   | <a href="#">ML702928</a> , The Macaulay Library    | <a href="#">[4]</a>                        |
| <i>Mareca falcata/Anas falcata</i>                 | 0.74 | 0.64900   | <a href="#">ML700864</a> , The Macaulay Library    | <a href="#">[4]</a>                        |
| <i>Lamprotornis superbus</i>                       | 0.59 | 0.06490   | <a href="#">ML701505</a> , The Macaulay Library    | <a href="#">[4]</a>                        |
| <i>Rhodospiza obsoleta</i>                         | 1.18 | 0.02550   | <a href="#">ML720078</a> , The Macaulay Library    | <a href="#">[4]</a>                        |
| <i>Alectoris rufa</i>                              | 0.55 | 0.52800   | <a href="#">ML720443</a> , The Macaulay Library    | <a href="#">[4]</a>                        |
| <i>Rynchops niger</i>                              | 0.53 | 0.30150   | <a href="#">ML487607</a> , The Macaulay Library    | <a href="#">[4]</a>                        |
| <i>Nyctanassa violacea</i> (2)                     | 0.47 | 0.68250   | <a href="#">ML487684</a> , The Macaulay Library    | <a href="#">[4]</a>                        |
| <i>Thalasseus maximus maximus</i>                  | 0.63 | 0.47000   | <a href="#">ML487811</a> , The Macaulay Library    | <a href="#">[4]</a>                        |
| <i>Calidris virgata</i>                            | 0.55 | 0.20150   | <a href="#">ML488445</a> , The Macaulay Library    | <a href="#">[4]</a>                        |
| <i>Egretta rufescens</i>                           | 0.42 | 0.61400   | <a href="#">ML488537</a> , The Macaulay Library    | <a href="#">[4]</a>                        |
| <i>Ardea herodias</i> [herodias Group]             | 0.60 | 2.29500   | <a href="#">ML487312</a> , The Macaulay Library    | <a href="#">[4]</a>                        |
| <i>Phoebastria immutabilis</i>                     | 0.67 | 3.15000   | <a href="#">ML485773</a> , The Macaulay Library    | <a href="#">[4]</a>                        |
| <i>Chlamydera cerviniventris</i>                   | 0.83 | 0.15650   | <a href="#">ML486483</a> , The Macaulay Library    | <a href="#">[4]</a>                        |
| <i>Leucophaeus atricilla</i>                       | 0.79 | 0.30800   | <a href="#">ML483554</a> , The Macaulay Library    | <a href="#">[4]</a>                        |
| <i>Fratercula arctica</i>                          | 0.64 | 0.38100   | <a href="#">ML483591</a> , The Macaulay Library    | <a href="#">[4]</a>                        |
| <i>Mergus merganser americanus</i>                 | 0.82 | 1.47050   | <a href="#">ML484047</a> , The Macaulay Library    | <a href="#">[4]</a>                        |
| <i>Parkesia motacilla</i>                          | 1.04 | 0.01990   | <a href="#">ML482406</a> , The Macaulay Library    | <a href="#">[4]</a>                        |
| <i>Alligator mississippiensis</i>                  | 3.15 | 225.50000 | <a href="#">Phil Lanoue</a>                        | <a href="#">[6]</a> , <a href="#">Link</a> |
| <i>Casuarus casuarius</i>                          | 0.48 | 44.00000  | <a href="#">ML303012171</a> , The Macaulay Library | <a href="#">[4]</a> , <a href="#">Link</a> |
| <i>Cophosaurus texanus</i>                         | 2.37 | 0.00423   | <a href="#">Sonoran Images</a>                     | <a href="#">[40]</a>                       |
| <i>Capreolus capreolus</i>                         | 0.34 | 26.00000  | <a href="#">biolib.cz</a>                          | <a href="#">[6]</a> , <a href="#">Link</a> |
| <i>Crocodylus johnstoni</i>                        | 1.05 | 20.90000  | <a href="#">[41]</a>                               | <a href="#">[41]</a>                       |
| <i>Marasuchus lilloensis</i>                       | 1.04 | 0.28800   | <a href="#">[41]</a>                               | <a href="#">[41]</a>                       |
| <i>Heterodontosaurus tucki</i>                     | 0.80 | 4.50000   | <a href="#">[41]</a>                               | <a href="#">[41]</a>                       |

**Table E1. Information on data collected for 364 animals.** Table with animal names, frontal aspect ratio, mass, and the source from where animal photograph and mass were obtained.

|                                    |      |             |      |      |
|------------------------------------|------|-------------|------|------|
| <i>Staurikosaurus pricei</i>       | 1.09 | 21.30000    | [41] | [41] |
| <i>Plateosaurus engelhardti</i>    | 1.16 | 753.00000   | [41] | [41] |
| <i>Coelophysis bauri</i>           | 1.16 | 18.30000    | [41] | [41] |
| <i>Dilophosaurus wetherilli</i>    | 0.86 | 462.00000   | [41] | [41] |
| <i>Allosaurus fragilis</i>         | 1.04 | 1340.00000  | [41] | [41] |
| <i>Tyrannosaurus rex</i> (2)       | 0.94 | 10800.00000 | [41] | [41] |
| <i>Struthiomimus sedens</i>        | 0.99 | 568.00000   | [41] | [41] |
| <i>cf. Caenagnathus</i>            | 1.30 | 12.50000    | [41] | [41] |
| <i>Velociraptor mongoliensis</i>   | 1.01 | 14.10000    | [41] | [41] |
| <i>Microraptor gui</i>             | 0.94 | 1.21000     | [41] | [41] |
| <i>Archaeopteryx lithographica</i> | 0.94 | 0.09920     | [41] | [41] |
| <i>Pengornis houi</i>              | 1.17 | 0.22900     | [41] | [41] |
| <i>Yixianornis grabaui</i>         | 0.84 | 0.20100     | [41] | [41] |
| <i>Gallus gallus</i>               | 0.58 | 2.57000     | [41] | [41] |

**Table E2. Information on terrain statistics.** Table showing the name of the site, the value of Hurst indices, the increment length, method of measurement of the terrain roughness, and the corresponding citation for the study.

| Site                                 | Information      | H1           | H2    | Breakpoint<br>mm | Scale                      | Method         | Citation |
|--------------------------------------|------------------|--------------|-------|------------------|----------------------------|----------------|----------|
| Cowra, Australia                     |                  | 0.7          |       |                  | 1 mm                       | Semivariogram  | [42]     |
| River-bed gravel, Field 1            |                  | 0.614        | 0.205 | 10 mm            | 0.003 m                    | Semivariogram  | [43]     |
| River-bed gravel, Field 2            |                  | 0.628        | 0.311 | 10 mm            | 0.003 m                    | Semivariogram  | [43]     |
| Flume 1, lab                         |                  | 0.647        |       |                  | 0.003 m                    | Semivariogram  | [43]     |
| Flume 2, lab                         |                  | 0.62         | 0.343 | 10 mm            | 0.003 m                    | Semivariogram  | [43]     |
| Flume 3, lab                         |                  | 0.613        | 0.334 | 10 mm            | 0.15 cm                    | Semivariogram  | [43]     |
| Full area flume, lab                 |                  | 0.647        | 0.239 | 10 mm            | 0.15 cm                    | Semivariogram  | [43]     |
| Semiarid grassland, New Mexico.      |                  | 0.20-0.05    |       |                  | 6.25 cm                    | Box counting   | [44]     |
| Moderately exposed shores, UK        |                  | 0.94         |       |                  | 1 mm                       | Semivariogram  | [45]     |
| Moderately exposed shores, Hong Kong |                  | 0.002, 0.082 |       |                  | 1 mm                       | Divider        | [46]     |
| Hermannsdorf (Upper Austria)         | Arable land      | 0.61         |       |                  | 12 $\mu$ m                 | Perimeter-area | [47]     |
| Hermannsdorf (Upper Austria)         | Arable land      | 0.74         |       |                  | 12 $\mu$ m                 | Perimeter-area | [47]     |
| Kaltenleutgeben (Lower Austria)      | Deciduous forest | 0.67         |       |                  | 12 $\mu$ m                 | Perimeter-area | [47]     |
| Kaltenleutgeben (Lower Austria)      | Deciduous forest | 0.68         |       |                  | 12 $\mu$ m                 | Perimeter-area | [47]     |
| Trautenfels (Styria)                 | Arable land      | 0.7          |       |                  | 12 $\mu$ m                 | Perimeter-area | [47]     |
| Oak (Quercu                          |                  | 0.8          |       |                  | [48]                       | Boundary grid  | [49]     |
| Spruce (Pice                         |                  | 0.25         |       |                  | [48]                       | Boundary grid  | [49]     |
| Lichen thali                         |                  | 0.42-0.41    |       |                  | 0.02 - 0.5 mm              | Boundary grid  | [50]     |
| Soil pore surface dimension          |                  | 0.39         |       |                  | 0.05 $\mu$ m               | Box counting   | [51]     |
| Moldboard ploughing                  |                  | 0.29         |       |                  | 1 - 3.52 m <sup>2</sup>    | Semivariogram  | [52]     |
| Chisel ploughing                     |                  | 0.37         |       |                  | 0.21 - 1.12 m <sup>2</sup> | Semivariogram  | [52]     |
| Moldboard ploughing                  |                  | 0.19         |       |                  | 0.21 - 1.12 m <sup>2</sup> | Semivariogram  | [52]     |
| Chisel ploughing                     |                  | 0.09         |       |                  | 0.21 - 1.12 m <sup>2</sup> | Semivariogram  | [52]     |
| Styria, Austria                      |                  | 0.62-0.66    |       |                  | 12 $\mu$ m                 | [47]           | [53]     |



**Table E2. Information on terrain statistics.** Table showing the name of the site, the value of Hurst indices, the increment length, method of measurement of the terrain roughness, and the corresponding citation for the study.

|                                                                |           |       |      |     |                                 |                |      |
|----------------------------------------------------------------|-----------|-------|------|-----|---------------------------------|----------------|------|
| A2 silty soil, 19%clay                                         |           | 0.1   |      |     | $10^{-3} - 10^{-5} \mu\text{m}$ | [54]           | [55] |
| A2g-B1g silty soil, 33% clay                                   |           | 0.31  |      |     | $10^{-3} - 10^{-5} \mu\text{m}$ | [54]           | [55] |
| A1b sandy soil                                                 |           | 0.25  |      |     | $10^{-3} - 10^{-5} \mu\text{m}$ | [54]           | [55] |
| England airport runway                                         |           | 0.5   |      |     | 30 cm lag                       | Power spectrum | [56] |
| Topographic heights france                                     |           | 0.5   |      |     | 10 m lag                        | Semivariogram  | [56] |
| Shadow mountain, Colorado                                      |           | 0.71  |      |     | 30 m                            | Semivariogram  | [57] |
| Mt Everest                                                     |           | 0.842 |      |     | 20 m                            | Semivariogram  | [57] |
| Barberry, <i>Berberis vulgaris</i> L.<br>(evergreen)           | Mag high  | 0.54  |      |     | 2 mm                            | Box counting   | [48] |
|                                                                | low       | 0.57  |      |     | 2 mm                            | Box counting   | [48] |
| Virginia creeper, <i>Parthenocissus</i><br><i>tricuspidata</i> | High      | 0.72  |      |     | 2 mm                            | Box counting   | [48] |
|                                                                | low       | 0.45  |      |     | 2 mm                            | Box counting   | [48] |
| Weeping elm, <i>Ulmus glabra</i><br><i>forma pendula</i>       | low       | 0.59  |      |     | 2 mm                            | Box counting   | [48] |
| Cotoneaster, <i>Cotoneaster hori-</i><br><i>zontalis</i>       | high      | 0.65  |      |     | 2 mm                            | Box counting   | [48] |
|                                                                | low       | 0.21  |      |     | 2 mm                            | Box counting   | [48] |
| Ivy, <i>Hedera helix</i> L                                     | low       | 0.61  |      |     | 2 mm                            | Box counting   | [48] |
| Yew, <i>Taxus baccata</i> L.                                   | high      | 0.53  |      |     | 2 mm                            | Box counting   | [48] |
|                                                                | low       | 0.32  |      |     | 2 mm                            | Box counting   | [48] |
| Silver birch, <i>Betula pendula</i>                            | medium    | 0.6   |      |     | 2 mm                            | Box counting   | [48] |
| Downy birch, <i>Betula pubescens</i><br>Ehrh                   | medium    | 0.6   |      |     | 2 mm                            | Box counting   | [48] |
| Ash, <i>Fraxinus excelsior</i> L                               | medium    | 0.58  |      |     | 2 mm                            | Box counting   | [48] |
| Sycamore, <i>Acer pseudoplatanus</i><br>L.                     | medium    | 0.69  |      |     | 2 mm                            | Box counting   | [48] |
| Ropy pahoehoe                                                  | DEC I (x) | 0.45  | 0.27 | 200 | 2.5 cm                          | Deviogram      | [58] |
| Ropy pahoehoe                                                  | DEC I (y) | 0.44  | 0.21 | 570 | 2.5 cm                          | Deviogram      | [58] |
| Sheet pahoehoe                                                 | DEC 2 (x) | 0.29  |      |     | 2.5 cm                          | Deviogram      | [58] |



**Table E2. Information on terrain statistics.** Table showing the name of the site, the value of Hurst indices, the increment length, method of measurement of the terrain roughness, and the corresponding citation for the study.

|                                                         |            |      |       |      |        |           |      |
|---------------------------------------------------------|------------|------|-------|------|--------|-----------|------|
| Sheet pahoehoe                                          | DEC 2 (y)  | 0.43 | 0.18  | 140  | 2.5 cm | Deviogram | [58] |
| Slab pahoehoe                                           | DEC 3 (x)  | 0.32 |       |      | 2.5 cm | Deviogram | [58] |
| Slab pahoehoe                                           | DEC 3 (y)  | 0.49 | 0.17  | 320  | 2.5 cm | Deviogram | [58] |
| Spiny pahoehoe                                          | DEC 4 (x)  | 0.39 |       |      | 2.5 cm | Deviogram | [58] |
| Spiny pahoehoe                                          | DEC 4 (y)  | 0.4  |       |      | 2.5 cm | Deviogram | [58] |
| Clinker a'a (85%) 10-50 cm in size                      | DEC 5 (x)  | 0.38 | 0.07  | 360  | 2.5 cm | Deviogram | [58] |
| and 15% transitional lava plates                        | DEC 5 (y)  | 0.26 | -0.02 | 310  | 2.5 cm | Deviogram | [58] |
| Ball a'a 30-130 cm in size with some clinker            | DEC 6 (x)  | 0.4  | 0.04  | 380  | 2.5 cm | Deviogram | [58] |
|                                                         | DEC 6 (y)  | 0.45 | 0.14  | 600  | 2.5 cm | Deviogram | [58] |
| Ball a'a (60%) 50-150 cm                                | DEC 7 (x)  | 0.55 | 0.14  | 340  | 2.5 cm | Deviogram | [58] |
| and clinker (35%) 5-25 cm                               | DEC 7 (y)  | 0.4  | 0.02  | 270  | 2.5 cm | Deviogram | [58] |
| Clinker a'a (65%) 10-70 cm and ball a'a (35%)           | DEC 8 (x)  | 0.38 |       |      | 2.5 cm | Deviogram | [58] |
|                                                         | DEC 8 (y)  | 0.41 | 0.05  | 360  | 2.5 cm | Deviogram | [58] |
| Clinker a'a (90%) uniform 5-20 cm                       | DEC 9 (x)  | 0.55 | 0.04  | 220  | 2.5 cm | Deviogram | [58] |
| and ball a'a (10%) 15-30 cm                             | DEC 9 (y)  | 0.39 | -0.01 | 210  | 2.5 cm | Deviogram | [58] |
| Clinker a'a (90%) 10-40 cm and ball a'a (10%) 40-120 cm | DEC 10 (x) | 0.42 | -0.07 | 220  | 2.5 cm | Deviogram | [58] |
|                                                         | DEC 10 (y) | 0.35 |       |      | 2.5 cm | Deviogram | [58] |
| Clinker a'a (85%) 20-50 cm and ball a'a (15%) 30-70 cm  | DEC 11 (x) | 0.32 |       |      | 2.5 cm | Deviogram | [58] |
|                                                         | DEC 11 (y) | 0.32 | 0.18  | 180  | 2.5 cm | Deviogram | [58] |
| Clinker a'a (85%) 20-50 cm and ball a'a (15%) 40-100 cm | DEC 12 (x) | 0.38 | 0.02  | 390  | 2.5 cm | Deviogram | [58] |
|                                                         | DEC 12 (y) | 0.31 |       |      | 2.5 cm | Deviogram | [58] |
| Ball a'a (50%) 30-130 cm and clinker                    | DEC 13 (x) | 0.28 |       |      | 2.5 cm | Deviogram | [58] |
| (40%) 5-30 cm, plates (10%)                             | DEC 13 (y) | 0.3  | -0.16 | 570  | 2.5 cm | Deviogram | [58] |
| Ponded pahoehoe                                         | KIL 1      | 0.65 | 0.07  | 5500 | 25 cm  | Deviogram | [58] |
| Ponded pahoehoe with Im tumuli                          | KIL 2      | 0.69 | 0.38  | 5000 | 25 cm  | Deviogram | [58] |

**Table E2. Information on terrain statistics.** Table showing the name of the site, the value of Hurst indices, the increment length, method of measurement of the terrain roughness, and the corresponding citation for the study.

|                                        |           |      |      |      |       |           |      |
|----------------------------------------|-----------|------|------|------|-------|-----------|------|
| Intermediate pahoehoe; tilted plates   | KIL 3     | 0.4  |      |      | 25 cm | Deviogram | [58] |
| Intermediate billowy pahoehoe          | KIL 4     | 0.43 | 0.18 | 4200 | 25 cm | Deviogram | [58] |
| Large, tilted, spiny plates; a'a flow  | KIL 5     | 0.24 | 0.4  | 2800 | 25 cm | Deviogram | [58] |
| Intermediate pahoehoe, similar to KIL4 | KIL 6     | 0.52 | 0.13 | 6800 | 25 cm | Deviogram | [58] |
| Channelized ropy pahoehoe              | KIL 7     | 0.68 |      |      | 25 cm | Deviogram | [58] |
| Platy pahoehoe with significant tilts  | KIL 8     | 0.41 | 0.07 | 8900 | 25 cm | Deviogram | [58] |
| Mostly small spiny plates, a'a flow    | KIL 9     | 0.28 |      |      | 25 cm | Deviogram | [58] |
| Sheet pahoehoe flow; ropy structure    | KIL 10    | 0.48 | 0.11 | 8200 | 25 cm | Deviogram | [58] |
| Smooth to intermediate pahoehoe        | KIL 11    | 0.59 |      |      | 25 cm | Deviogram | [58] |
| Very smooth thin-lobed pahoehoe        | KIL 15    | 0.66 | 0.41 | 1300 | 25 cm | Deviogram | [58] |
| Devils Golf Course:                    | DV12 (x)  | 0.62 | 0.11 | 250  | 1 cm  | Deviogram | [58] |
| Eroded, silty salt                     | DV12 (y)  | 0.64 | 0.32 | 180  | 1 cm  | Deviogram | [58] |
| Trail Canyon alluvial fan:             | DV15 (x)  | 0.52 | 0.17 | 70   | 1 cm  | Deviogram | [58] |
| Intermediate age, active surface       | DV15 (y)  | 0.56 | 0.29 | 70   | 1 cm  | Deviogram | [58] |
| Flood plain surface:                   | DV 18 (x) | 0.62 | 0.37 | 70   | 1 cm  | Deviogram | [58] |
| Central death valley                   | DV 18 (y) | 0.31 | 0.45 | 30   | 1 cm  | Deviogram | [58] |
| Mars Hill, eroded fanglomerate         | DV22 (x)  | 0.5  | 0.04 | 1030 | 1 cm  | Deviogram | [58] |
|                                        | DV22 (y)  | 0.58 | 0.35 | 130  | 1 cm  | Deviogram | [58] |
| Mars Hill, eroded fanglomerate         | DV24 (x)  | 0.55 | 0.32 | 220  | 1 cm  | Deviogram | [58] |
|                                        | DV24 (y)  | 0.53 | 0.32 | 70   | 1 cm  | Deviogram | [58] |
| Mars Hill, eroded fanglomerate         | DV25 (x)  | 0.63 | 0.33 | 130  | 1 cm  | Deviogram | [58] |
|                                        | DV25 (y)  | 0.53 | 0.11 | 360  | 1 cm  | Deviogram | [58] |

**Table E2. Information on terrain statistics.** Table showing the name of the site, the value of Hurst indices, the increment length, method of measurement of the terrain roughness, and the corresponding citation for the study.

|                                                       |           |      |      |     |      |           |      |
|-------------------------------------------------------|-----------|------|------|-----|------|-----------|------|
| Active dunes near Stovepipe Wells                     | DV29 (x)  | 0.3  | 0.12 | 590 | 1 cm | Deviogram | [58] |
|                                                       | DV29 (y)  | 0.38 |      |     | 1 cm | Deviogram | [58] |
| Kit Fox alluvial fan:                                 | DV36 (x)  | 0.51 | 0.18 | 30  | 1 cm | Deviogram | [58] |
| young, inactive surface                               | DV36 (y)  | 0.6  | 0.25 | 30  | 1 cm | Deviogram | [58] |
| Stovepipe Wells alluvial fan at east edge of dunes    | DV39 (x)  | 0.42 | 0.19 | 30  | 1 cm | Deviogram | [58] |
|                                                       | DV39 (y)  | 0.34 | 0.21 | 10  | 1 cm | Deviogram | [58] |
| Older basalt flow with silt mantle, northern LCVF     | LC08 (x)  | 0.41 | 0.18 | 320 | 1 cm | Deviogram | [58] |
|                                                       | LC08(y)   | 0.56 | 0.36 | 50  | 1 cm | Deviogram | [58] |
| Older basalt flow with silt mantle, northern LCVF     | LC11 (x)  | 0.46 | 0.16 | 80  | 1 cm | Deviogram | [58] |
|                                                       | LC11 (y)  | 0.56 | 0.28 | 70  | 1 cm | Deviogram | [58] |
| Older basalt flow with silt mantle, northern LCVF     | LC13(x)   | 0.43 | 0.05 | 670 | 1 cm | Deviogram | [58] |
|                                                       | LC13 (y)  | 0.48 | 0.14 | 270 | 1 cm | Deviogram | [58] |
| Black Rock a'a flow, young northern lobe              | LC17 (x)  | 0.58 |      |     | 1 cm | Deviogram | [58] |
|                                                       | LC17 (y)  | 0.53 |      |     | 1 cm | Deviogram | [58] |
| Black Rock a'a flow, young southern lobe              | LC23 (x)  | 0.56 | 0.41 | 60  | 1 cm | Deviogram | [58] |
|                                                       | LC23 (y)  | 0.68 | 0.38 | 70  | 1 cm | Deviogram | [58] |
| Black Rock a'a flow, young silt-mantled southern lobe | LC25 (x)  | 0.61 | 0.37 | 110 | 1 cm | Deviogram | [58] |
|                                                       | LC25 (y)  | 0.69 | 0.42 | 70  | 1 cm | Deviogram | [58] |
| Black Rock a'a flow, young silt-mantled southern lobe | LC27 (x)  | 0.55 | 0.2  | 100 | 1 cm | Deviogram | [58] |
|                                                       | LC27 (y)  | 0.67 | 0.36 | 60  | 1 cm | Deviogram | [58] |
| Black Rock a'a flow, young silt-mantled southern lobe | LC29 (x)  | 0.6  | 0.36 | 70  | 1 cm | Deviogram | [58] |
|                                                       | LC29 (y)  | 0.64 | 0.29 | 70  | 1 cm | Deviogram | [58] |
| Lunar Lake Playa, LCVF northern end of playa          | LC39 (x)  | 0.42 | 0.13 | 40  | 1 cm | Deviogram | [58] |
|                                                       | LC39 (y)  | 0.59 | 0.22 | 50  | 1 cm | Deviogram | [58] |
| Lunar Lake Playa, LCVF middle of playa                | LC43 (x)  | 0.47 | 0.12 | 80  | 1 cm | Deviogram | [58] |
|                                                       | LC43 (y)  | 0.49 | 0.26 | 70  | 1 cm | Deviogram | [58] |
| Lunar Lake Playa, LCVF southern end                   | LC47 (x)  | 0.46 | 0.1  | 240 | 1 cm | Deviogram | [58] |
|                                                       | LC47 (y)  | 0.53 | 0.09 | 240 | 1 cm | Deviogram | [58] |
| Lunar Lake Playa, LCVF                                | LC 52 (x) | 0.55 | 0.16 | 460 | 1 cm | Deviogram | [58] |

**Table E2. Information on terrain statistics.** Table showing the name of the site, the value of Hurst indices, the increment length, method of measurement of the terrain roughness, and the corresponding citation for the study.

|                                                   |           |      |      |      |       |               |      |
|---------------------------------------------------|-----------|------|------|------|-------|---------------|------|
| model site for GRSFE                              | LC52 (y)  | 0.49 | 0.16 | 510  | 1 cm  | Deviogram     | [58] |
| Intermediate age basalt flow,                     | LC58 (x)  | 0.33 | 0.02 | 420  | 1 cm  | Deviogram     | [58] |
| adjacent to playa, GRSFE model site               | LC58 (y)  | 0.64 | 0.18 | 60   | 1 cm  | Deviogram     | [58] |
| Intermediate age basalt flow,                     | LC59 (x)  | 0.63 | 0.21 | 60   | 1 cm  | Deviogram     | [58] |
| adjacent to playa, GRSFE model site               | LC59 (y)  | 0.64 | 0.24 | 50   | 1 cm  | Deviogram     | [58] |
| Intermediate age basalt flow,                     | LC60 (x)  | 0.54 | 0.16 | 50   | 1 cm  | Deviogram     | [58] |
| adjacent to playa, GRSFE model site               | LC60 (y)  | 0.58 | 0.22 | 40   | 1 cm  | Deviogram     | [58] |
| Intermediate age basalt flow                      | LC65 (x)  | 0.52 | 0.23 | 40   | 1 cm  | Deviogram     | [58] |
| northeast of Lunar Crater                         | LC65 (y)  | 0.59 | 0.12 | 40   | 1 cm  | Deviogram     | [58] |
| Obsidian Dome, vent region with megablocks        | ID40 (x)  | 0.52 |      |      | 25 cm | Deviogram     | [58] |
|                                                   | ID40 (y)  | 0.42 |      |      | 25 cm | Deviogram     | [58] |
| Wilson Dome, vent region with heavy tephra mantle | ID180 (x) | 0.42 |      |      | 25 cm | Deviogram     | [58] |
|                                                   | ID180 (y) | 0.37 |      |      | 25 cm | Deviogram     | [58] |
| Obsidian Dome, ridged                             | ID210 (x) | 0.42 |      |      | 25 cm | Deviogram     | [58] |
|                                                   | ID210 (y) | 0.38 |      |      | 25 cm | Deviogram     | [58] |
| Obsidian Dome, ridged                             | ID230 (x) | 0.47 |      |      | 25 cm | Deviogram     | [58] |
|                                                   | ID230 (y) | 0.32 |      |      | 25 cm | Deviogram     | [58] |
| Obsidian Dome,jumbled                             | ID250 (x) | 0.53 |      |      | 25 cm | Deviogram     | [58] |
|                                                   | ID250 (y) | 0.49 | 0.04 | 1260 | 25 cm | Deviogram     | [58] |
| Thick, blocky, andesitic flow                     | SB1       | 0.4  |      |      | 3 m   | Deviogram     | [58] |
| Thick, blocky, andesitic flow                     | SB2       | 0.47 |      |      | 3 m   | Deviogram     | [58] |
| Thick, blocky, andesitic flow                     | SB3       | 0.5  |      |      | 3 m   | Deviogram     | [58] |
| Thick, blocky, andesitic flow                     | SB4       | 0.5  |      |      | 3 m   | Deviogram     | [58] |
| Thick, blocky, andesitic flow                     | SB5       | 0.29 |      |      | 3 m   | Deviogram     | [58] |
| Fallow plots                                      | Rion      | 0.66 |      |      | 1 mm  | Semivariogram | [59] |
|                                                   | Pacolet   | 0.4  |      |      | 1 mm  | Semivariogram | [59] |

**Table E2. Information on terrain statistics.** Table showing the name of the site, the value of Hurst indices, the increment length, method of measurement of the terrain roughness, and the corresponding citation for the study.

|                          |               |            |  |  |          |                     |      |
|--------------------------|---------------|------------|--|--|----------|---------------------|------|
| soil 1                   | Smooth        | 0.54       |  |  | 1 mm     | Semivariogram       | [60] |
| soil 2                   | Cloddy, Sowed | 0.65       |  |  | 1 mm     | Semivariogram       | [60] |
| soil 3                   | Medium rough  | 0.7        |  |  | 1 mm     | Semivariogram       | [60] |
| soil 4                   | Ploughed      | 0.79       |  |  | 1 mm     | Semivariogram       | [60] |
| Conventional, fallow     |               | 0.44       |  |  | 1 mm     | Semivariogram       | [60] |
| Conventional, soybean    |               | 0.48       |  |  | 1 mm     | Semivariogram       | [60] |
| Chisel+Échain, fallow    |               | 0.43       |  |  | 2 mm     | Semivariogram       | [61] |
| Chisel+Échain, soybean   |               | 0.42       |  |  | 2 mm     | Semivariogram       | [61] |
| Chisel, fallow           |               | 0.47       |  |  | 2 mm     | Semivariogram       | [61] |
| Chisel, soybean          |               | 0.49       |  |  | 2 mm     | Semivariogram       | [61] |
| Lower Saxony             |               | 0.6        |  |  | 50 cm    | Power spectra       | [62] |
| Kilauea volcano          | Site A        | 0.28       |  |  | 2 - 3 cm | 2D roughness method | [63] |
|                          | Site B        | 0.47       |  |  | 2 - 3 cm | 2D roughness method | [63] |
|                          | Site C        | 0.51       |  |  | 2 - 3 cm | 2D roughness method | [63] |
|                          | Site D        | 0.78       |  |  | 2 - 3 cm | 2D roughness method | [63] |
|                          | Site E        | 0.5        |  |  | 2 - 3 cm | 2D roughness method | [63] |
|                          | Site F        | 0.67       |  |  | 2 - 3 cm | 2D roughness method | [63] |
| Coastal Plain            | USA           | 0.35       |  |  | 30 m     | Semivariogram       | [64] |
| Blue Ridge               | USA           | 0.68       |  |  | 30 m     | Semivariogram       | [64] |
| Valley and ridge         | USA           | 0.64       |  |  | 30 m     | Semivariogram       | [64] |
| Appalachian plateaus     | USA           | 0.7        |  |  | 30 m     | Semivariogram       | [64] |
| Interior low plateaus    | USA           | 0.59       |  |  | 30 m     | Semivariogram       | [64] |
| Colorado plateaus        | USA           | 0.66       |  |  | 30 m     | Semivariogram       | [64] |
| Basin and range          | USA           | 0.71       |  |  | 30 m     | Semivariogram       | [64] |
| Burwash Wealdon          | NW            | 0.83, 0.48 |  |  | 50 m     | Semivariogram       | [65] |
|                          | SW            | 0.88, 0.54 |  |  | 50 m     | Semivariogram       | [65] |
| Billingshurst Weald Clay | NW            | 0.80, 0.45 |  |  | 50 m     | Semivariogram       | [65] |
|                          | SW            | 0.85, 0.42 |  |  | 50 m     | Semivariogram       | [65] |
| Singleton Chalk          | NW            | 0.81, 0.44 |  |  | 50 m     | Semivariogram       | [65] |
|                          | SW            | 0.78       |  |  | 50 m     | Semivariogram       | [65] |

**Table E2. Information on terrain statistics.** Table showing the name of the site, the value of Hurst indices, the increment length, method of measurement of the terrain roughness, and the corresponding citation for the study.

|                               |         |            |  |  |      |               |      |
|-------------------------------|---------|------------|--|--|------|---------------|------|
| High Wycombe Chalk            | NW      | 0.75       |  |  | 50 m | Semivariogram | [65] |
|                               | SW      | 0.92       |  |  | 50 m | Semivariogram | [65] |
| Popham Chalk                  | NW      | 0.87, 0.42 |  |  | 50 m | Semivariogram | [65] |
|                               | SW      | 0.85, 0.52 |  |  | 50 m | Semivariogram | [65] |
| Lambourn Chalk                | NW      | 0.91       |  |  | 50 m | Semivariogram | [65] |
|                               | SW      | 0.81       |  |  | 50 m | Semivariogram | [65] |
| Egdon Heath Chalk             | NW      | 0.80, 0.52 |  |  | 50 m | Semivariogram | [65] |
|                               | SW      | 0.9        |  |  | 50 m | Semivariogram | [65] |
| Dartmoor Granite              | NW      | 0.9, 0.62  |  |  | 50 m | Semivariogram | [65] |
|                               | SW      | 0.91, 0.66 |  |  | 50 m | Semivariogram | [65] |
| Tavistock Culm                | NW      | 0.74       |  |  | 50 m | Semivariogram | [65] |
|                               | SW      | 0.74       |  |  | 50 m | Semivariogram | [65] |
| Stewkley U. Jurassic          | NW      | 0.86, 0.24 |  |  | 50 m | Semivariogram | [65] |
|                               | SW      | 0.87, 0.47 |  |  | 50 m | Semivariogram | [65] |
| Stow M. Jurassic              | NW      | 0.86       |  |  | 50 m | Semivariogram | [65] |
|                               | SW      | 0.86       |  |  | 50 m | Semivariogram | [65] |
| Ribbesdon L. Jurassic         | NW      | 0.85, 0.61 |  |  | 50 m | Semivariogram | [65] |
|                               | SW      | 0.84       |  |  | 50 m | Semivariogram | [65] |
| Forest of Wyre Coal Measures  | NW      | 0.73, 0.40 |  |  | 50 m | Semivariogram | [65] |
|                               | SW      | 0.88, 0.62 |  |  | 50 m | Semivariogram | [65] |
| Clun Forest Silurian          | NW      | 0.92, 0.66 |  |  | 50 m | Semivariogram | [65] |
|                               | SW      | 0.86       |  |  | 50 m | Semivariogram | [65] |
| Shelve P-Cam-Ord              | NW      | 0.85, 0.38 |  |  | 50 m | Semivariogram | [65] |
|                               | SW      | 0.92, 0.39 |  |  | 50 m | Semivariogram | [65] |
| Furtwangen (Bavaria)          | NW      | 0.89, 0.50 |  |  | 50 m | Semivariogram | [65] |
|                               | SW      | 0.90, 0.63 |  |  | 50 m | Semivariogram | [65] |
| Schleiden (Eifel)             | NW      | 0.80, 0.60 |  |  | 50 m | Semivariogram | [65] |
|                               | SW      | 0.81, 0.28 |  |  | 50 m | Semivariogram | [65] |
| USA                           |         | 0.61       |  |  | 90 m | Power spectra | [62] |
| Global continental topography | GTOPO30 | 0.6        |  |  | 1 km | Power spectra | [62] |

## References

- [1] Don E Wilson and Russell A Mittermeier, editors. *Handbook of the mammals of the world, Vol. 2. Hoofed Mammals*. Lynx Ediciones, Barcelona, 2011.
- [2] DE Wilson and RA Mittermeier, editors. *Handbook of Mammals of the World. Vol. 5. Monotremes and Marsupials*. Lynx Ediciones, Barcelona, 2015.
- [3] Frank E Zachos. *Handbook of the Mammals of the World. Vol. 8. Insectivores, Sloths and Colugos*. Springer, 2019.
- [4] John B Dunning Jr. *CRC handbook of avian body masses*. CRC press, 2007.
- [5] Cynthia S Parr, Mr Nathan Wilson, Mr Patrick Leary, Katja S Schulz, Ms Kristen Lans, Ms Lisa Walley, Jennifer A Hammock, Mr Anthony Goddard, Mr Jeremy Rice, Mr Marie Studer, et al. The encyclopedia of life v2: providing global access to knowledge about life on earth. *Biodiversity data journal*, (2), 2014.
- [6] P. Myers, R. Espinosa, C. S. Parr, T. Jones, G. S. Hammond, and T. A. Dewey. The animal diversity web (online), 2021. URL <https://animaldiversity.org>.
- [7] Claudia P Ceballos, Daniel Zapata, Carolina Alvarado, and Eisinhow Rincón. Morphology, diet, and population structure of the southern white-lipped mud turtle kinosternon leucostomum postinguinale (testudines: Kinosternidae) in the nus river drainage, colombia. *Journal of Herpetology*, 50(3):374–380, 2016.
- [8] Bog turtle. URL <https://web.archive.org/web/20210512151841/https://portal.ct.gov/DEEP/Wildlife/Fact-Sheets/Bog-Turtle>.
- [9] Antoine Louchart and Cécile Mourer-Chauviré. The dodo was not so slim: leg dimensions and scaling to body mass. *Naturwissenschaften*, 98(4):357–358, 2011.
- [10] Edwin Harris Colbert. The weights of dinosaurs. *American Museum Novitates*, (2076):1–16, 1962.
- [11] Jan Peczki. Implications of body-mass estimates for dinosaurs. *Journal of Vertebrate Paleontology*, 14(4):520–533, 1995.
- [12] Don E Wilson and Russell A Mittermeier, editors. *Handbook of the Mammals of the World. Vol. 1. Carnivores*. Lynx Ediciones, Barcelona, 2009.
- [13] Great barred frog (mixophyes fasciolatus) with chytridiomycosis and mycobacteriosis, 2016. URL <https://web.archive.org/web/20210206130654/https://arwh.org/interesting-cases/blog/great-barred-frog-mixophyes-fasciolatus-chytridiomycosis-and-mycobacteriosis#:~:text=Exterior%20findings%3A%20Weight%2025g>.
- [14] Franco Andreone, Paolo Eusebio Bergò, Vincenzo Mercurio, and Gonçalo M Rosa. Spatial ecology of scaphiophryne gottlebei in the canyons of the isalo massif, madagascar. *Herpetologica*, 69(1): 11–21, 2013.
- [15] Robert Andrew Balfour. *Differences in the growth of the wolf spider Hogna helluo (Araneae: Lycosidae) reared under high and low food quantity diets*. PhD thesis, Miami University, 2004.
- [16] N. Collar and P. F. D. Boesman. Blue-crowned lorikeet (vini australis), version 1.0. in birds of the world. URL <https://birdsoftheworld.org/bow/species/blclor2/cur/introduction>.



- [17] Leigh A Clayton, Jessica Nelson, Mark E Payton, John J McDonnell, Benjamin H Rossi, Kerry King-Rahn, and Dan Woodburn. Clinical signs, management, and outcome of presumptive ivermectin overdose in a group of dendrobatid frogs. *Journal of Herpetological Medicine and Surgery*, 22(1-2):5–11, 2012.
- [18] M. H. B. M. Salleh and S. A. B. M. Sah. Morphometric variations in distinguishing sex differences of river terrapin–batagur affinis. *Malayan Nature Journal*, 71(4):413–422, 2019.
- [19] MALCOLM S GORDON. Osmotic regulation in the green toad (bufo viridis). *Journal of Experimental Biology*, 39(2):261–270, 1962.
- [20] TR Birkhead, KE Lee, and P Young. Sexual cannibalism in the praying mantis hierodula membranacea. *Behaviour*, 106(1-2):112–118, 1988.
- [21] Wen-San Huang, Jun-Yi Lin, and John Yu-Lin Yu. Male reproductive cycle of the toad bufo melanostictus in taiwan. *Zoological Science*, 14(3):497–503, 1997.
- [22] Margaret E Janowski-Bell and Norman V Horner. Movement of the male brown tarantula, aphonopelma hentzi (araneae, theraphosidae), using radio telemetry. *Journal of Arachnology*, pages 503–512, 1999.
- [23] Sacramento Zoo. Solomon island leaf frog: Ceratobatrachus guentheri, 12 2016. URL <https://web.archive.org/web/20210512151018/https://www.saczoo.org/wp-content/uploads/2016/12/Solomon-Island-Leaf-Frog-Factsheet.pdf>.
- [24] RH Kaplan. Developmental plasticity and maternal effects of reproductive characteristics in the frog, bombina orientalis. *Oecologia*, 71(2):273–279, 1987.
- [25] Towa Olivier William Kamgaing, Kadiri Serge Bobo, Daniel Djekda, Keumbeng Blondel Vasco Azobou, Bobo René Hamadjida, Moaga Yannick Balangounde, Kamdem Joel Simo, and Hirokazu Yasuoka. Population density estimates of forest duikers (philantomba monticola & cephalophus spp.) differ greatly between survey methods. *African Journal of Ecology*, 56(4):908–916, 2018.
- [26] Asier Larramendi. Shoulder height, body mass, and shape of proboscideans. *Acta Palaeontologica Polonica*, 61(3):537–574, 2015.
- [27] John H Ostrom. *Osteology of Deinonychus antirrhopus, an unusual theropod from the Lower Cretaceous of Montana*. Yale Peabody Museum, 2019.
- [28] Delphine Angst, Eric Buffetaut, and Anick Abourachid. The end of the fat dodo? a new mass estimate for raphus cucullatus. *Naturwissenschaften*, 98(3):233–236, 2011.
- [29] Richard A Fariña. Limb bone strength and habits in large glyptodonts. *Lethaia*, 28(3):189–196, 1995.
- [30] Bruce J MacFadden. Fossil horses from "eohippus"(hyracotherium) to equus: scaling, cope's law, and the evolution of body size. *Paleobiology*, pages 355–369, 1986.
- [31] Ron A Moen, John Pastor, and Yosef Cohen. Antler growth and extinction of irish elk. *Evolutionary Ecology Research*, 1(2):235–249, 1999.
- [32] Alfred Sherwood Romer, Larry W Price, and Llewellyn Ivor Price. *Review of the Pelycosauria*, volume 28. Geological Society of America, 1940.
- [33] Nicolás E Campione. Extrapolating body masses in large terrestrial vertebrates. *Paleobiology*, 43(4):693–699, 2017.



- [34] Donald M Henderson. Pterosaur body mass estimates from three-dimensional mathematical slicing. *Journal of Vertebrate Paleontology*, 30(3):768–785, 2010.
- [35] Charlotte A Brassey, Susannah CR Maidment, and Paul M Barrett. Body mass estimates of an exceptionally complete stegosaurus (ornithischia: Thyreophora): comparing volumetric and linear bivariate mass estimation methods. *Biology letters*, 11(3):20140984, 2015.
- [36] James O Farlow, Matt B Smith, and John M Robinson. Body mass, bone “strength indicator,” and cursorial potential of tyrannosaurus rex. *Journal of Vertebrate Paleontology*, 15(4):713–725, 1995.
- [37] Michael R Voorhies and Joseph R Thomasson. Fossil grass anthoecia within miocene rhinoceros skeletons: diet in an extinct species. *Science*, 206(4416):331–333, 1979.
- [38] Richard H Yahner. Weight change, survival rate and home range change in the box turtle, terrapene carolina. *Copeia*, 1974(2):546–548, 1974.
- [39] Bianca Hohn-Schulte, Holger Preuschoft, Ulrich Witzel, and Claudia Distler-Hoffmann. Biomechanics and functional preconditions for terrestrial lifestyle in basal tetrapods, with special consideration of tiktaalik roseae. *Historical Biology*, 25(2):167–181, 2013.
- [40] Fred Punzo. Tail autotomy and running speed in the lizards cophosaurus texanus and uma notata. *Journal of Herpetology*, 16(3):329–331, 1982.
- [41] Vivian Allen, Karl T Bates, Zhiheng Li, and John R Hutchinson. Linking the evolution of body shape and locomotor biomechanics in bird-line archosaurs. *Nature*, 497(7447):104–107, 2013.
- [42] John C Gallant, Ian D Moore, Michael F Hutchinson, and Paul Gessler. Estimating fractal dimension of profiles: a comparison of methods. *Mathematical Geology*, 26(4):455–481, 1994.
- [43] Justin B Butler, Stuart N Lane, and Jim H Chandler. Characterization of the structure of river-bed gravels using two-dimensional fractal analysis. *Mathematical geology*, 33(3):301–330, 2001.
- [44] John A Wiens and Bruce T Milne. Scaling of ‘landscapes’ in landscape ecology, or, landscape ecology from a beetle’s perspective. *Landscape ecology*, 3(2):87–96, 1989.
- [45] Natalie J Frost, Michael T Burrows, Mark P Johnson, Mick E Hanley, and Stephen J Hawkins. Measuring surface complexity in ecological studies. *Limnology and Oceanography: Methods*, 3(4):203–210, 2005.
- [46] Vladimir E Kostylev, Johan Erlandsson, Mak Yiu Ming, and Gray A Williams. The relative importance of habitat complexity and surface area in assessing biodiversity: fractal application on rocky shores. *Ecological Complexity*, 2(3):272–286, 2005.
- [47] Ch Kampichler and M Hauser. Roughness of soil pore surface and its effect on available habitat space of microarthropods. In *Soil Structure/Soil Biota Interrelationships*, pages 223–232. Elsevier, 1993.
- [48] David R Morse, JH Lawton, MM Dodson, and MH Williamson. Fractal dimension of vegetation and the distribution of arthropod body lengths. *Nature*, 314(6013):731–733, 1985.
- [49] B Gunnarsson. Fractal dimension of plants and body size distribution in spiders. *Functional Ecology*, pages 636–641, 1992.
- [50] B Shorrocks, J Marsters, I Ward, and PJ Evennett. The fractal dimension of lichens and the distribution of arthropod body lengths. *Functional Ecology*, pages 457–460, 1991.
- [51] A Dathe, S Eins, J Niemeyer, and G Gerold. The surface fractal dimension of the soil–pore interface as measured by image analysis. *Geoderma*, 103(1-2):203–229, 2001.

- [52] E Vidal Vázquez, JG Vivas Miranda, and A Paz González. Characterizing anisotropy and heterogeneity of soil surface microtopography using fractal models. *Ecological Modelling*, 182(3-4): 337–353, 2005.
- [53] Christian Kampichler. Biomass distribution of a microarthropod community in spruce forest soil. *Biology and fertility of soils*, 19(2):263–265, 1995.
- [54] WI Friesen and RJ Mikula. Fractal dimensions of coal particles. *Journal of Colloid and Interface Science*, 120(1):263–271, 1987.
- [55] F Bartoli, R Philippy, M Doirisse, S Niquet, and M Dubuit. Structure and self-similarity in silty and sandy soils: the fractal approach. *Journal of Soil Science*, 42(2):167–185, 1991.
- [56] Peter A Burrough. Fractal dimensions of landscapes and other environmental data. *Nature*, 294 (5838):240–242, 1981.
- [57] Keith C Clarke and Diane M Schweizer. Measuring the fractal dimension of natural surfaces using a robust fractal estimator. *Cartography and Geographic Information Systems*, 18(1):37–47, 1991.
- [58] Michael K Shepard, Bruce A Campbell, Mark H Bulmer, Tom G Farr, Lisa R Gaddis, and Jeffrey J Plaut. The roughness of natural terrain: A planetary and remote sensing perspective. *Journal of Geophysical Research: Planets*, 106(E12):32777–32795, 2001.
- [59] Chi-hua Huang and Joe M Bradford. Applications of a laser scanner to quantify soil microtopography. *Soil Science Society of America Journal*, 56(1):14–21, 1992.
- [60] Mehrez Zribi, V Ciarletti, O Taconet, J Paillé, and P Boissard. Characterisation of the soil structure and microwave backscattering based on numerical three-dimensional surface representation: Analysis with a fractional brownian model. *Remote sensing of environment*, 72(2):159–169, 2000.
- [61] Flavio Luiz Foletto Eltz and L Darrell Norton. Surface roughness changes as affected by rainfall erosivity, tillage, and canopy cover. *Soil Science Society of America Journal*, 61(6):1746–1755, 1997.
- [62] J-S Gagnon, S Lovejoy, and D Schertzer. Multifractal earth topography. *Nonlinear Processes in Geophysics*, 13(5):541–570, 2006.
- [63] Aisha R Morris, F Scott Anderson, Peter J Mougini-Mark, Albert FC Haldemann, Benjamin A Brooks, and James Foster. Roughness of hawaiian volcanic terrains. *Journal of Geophysical Research: Planets*, 113(E12), 2008.
- [64] Brian Klinkenberg and MF Goodchild. The fractal properties of topography: a comparison of methods. *Earth surface processes and landforms*, 17(3):217–234, 1992.
- [65] WEH Culling and Mark Datko. The fractal geometry of the soil—covered landscape. *Earth Surface Processes and Landforms*, 12(4):369–385, 1987.
